# Supplementary material for: Scaling Motion Forecasting Models with Ensemble Distillation
Source: arXiv:2404.03843 source file (2024-05-13)
Supplement: Supplementary file 1 [file fig1.pdf]

Single Model

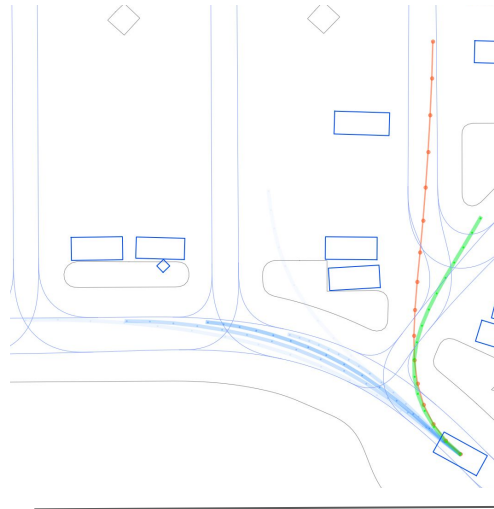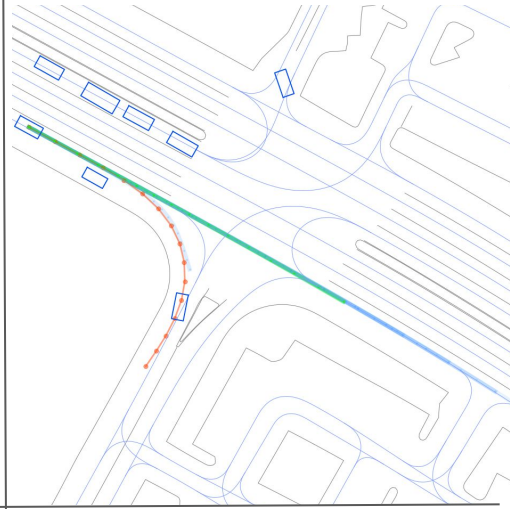

Ensemble

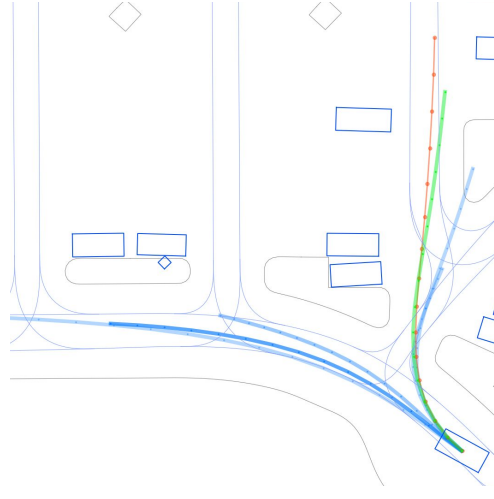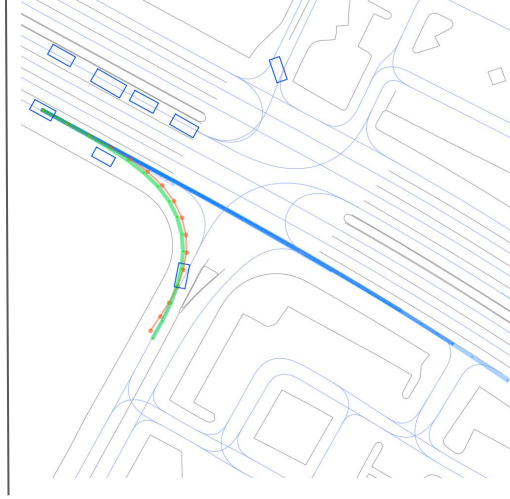

Supplementary

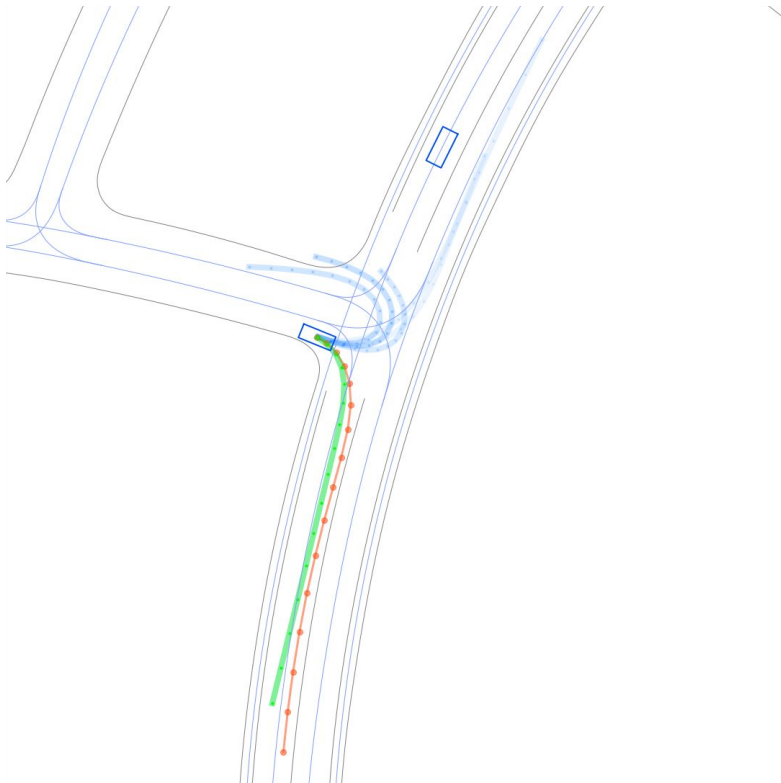

Single Model

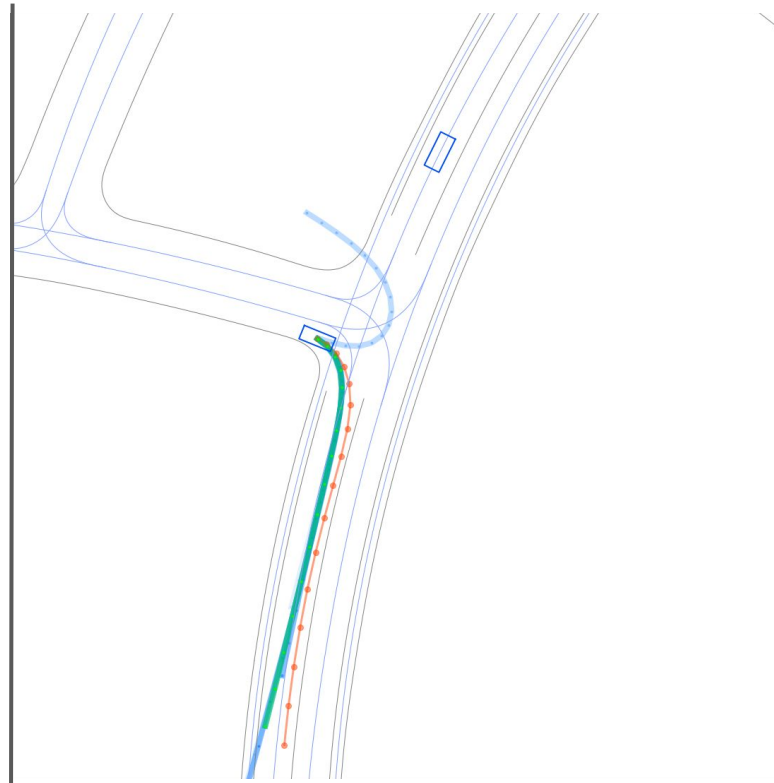

Ensemble

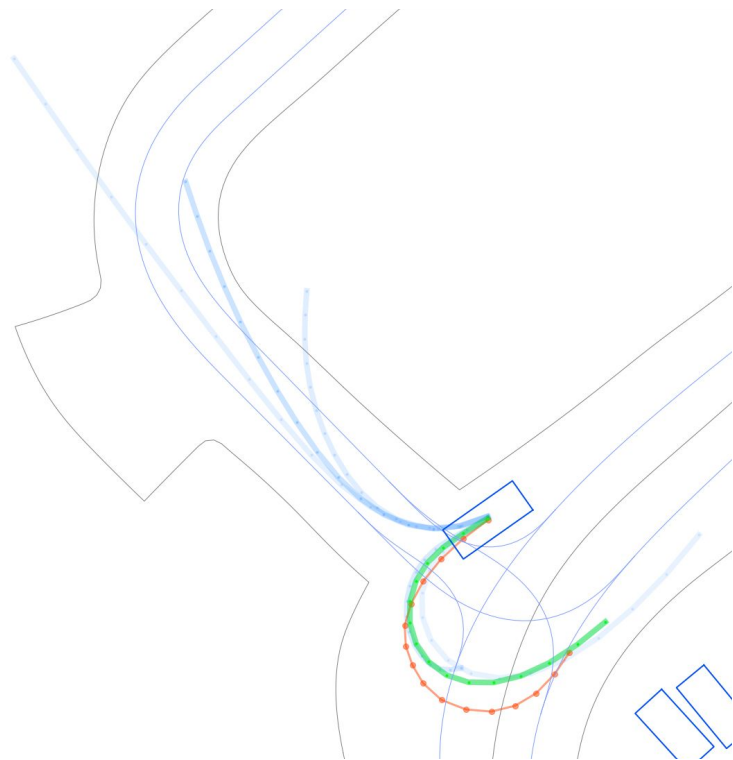

Single Model

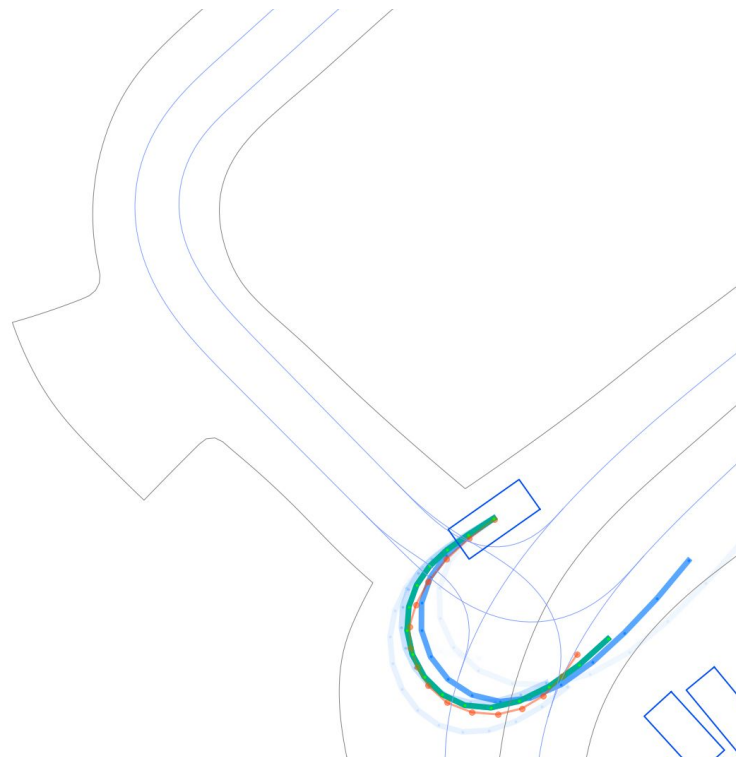

Ensemble

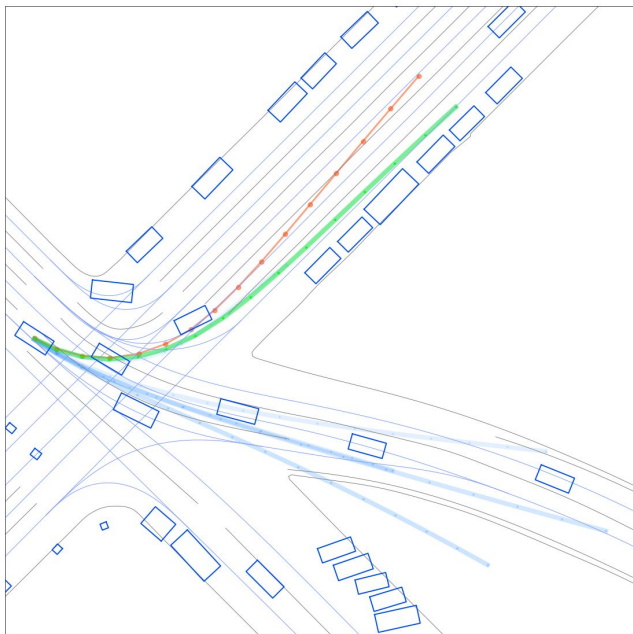

Single Model

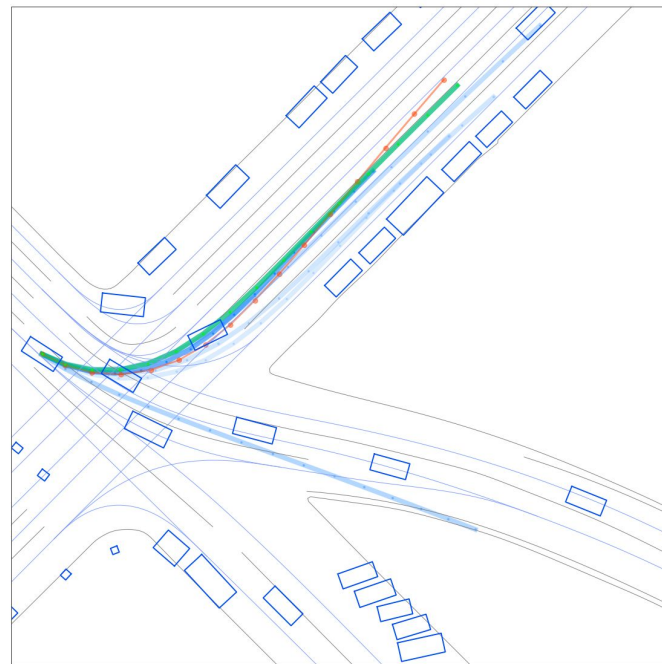

Ensemble

Single Model

Ensemble
